# Supplementary material for: Numerical Computation of Weil-Peterson Geodesics in the Universal Teichm\"uller Space
Source: arXiv:1307.2358 source file (2015-10-14)
Supplement: Supplementary file 1 [file appendix-periodic-stein.tex]

\section{Derivation of periodic Stein $WP$ norm}
\label{sec:periodic-stein}
Let $f: S^1 \rightarrow \R$ be a smooth function in $L^2_p$, the space of
periodic $L^2$ functions on $S^1$. We have already discussed how the $W P$ norm on $S^1$ is
given by \eqref{eq:wp-norm-fourier}.

Let $\omega^{(\alpha,\beta)}(r) = (1-r)^\alpha (1+r)^\beta$ for $r \in (-1,1)$
be the Jacobi polynomial weight function. The degree-$n$ Jacobi polynomial is
denoted $p_n^{(\alpha,\beta)}$ for all $\alpha,\beta>-1$ and $n \in \N_0$. Let
$L^2_{(\alpha,\beta)} \doteq L^2_{\omega^{(\alpha,\beta)}}$ and $\langle \cdot,
\cdot \rangle_{(\alpha,\beta)} \doteq \langle \cdot, \cdot
\rangle_{\omega^{(\alpha,\beta)}}$. We choose the (non-classical) convention
that the polynomials are normalized so that they are
$L^2_{(\alpha,\beta)}$-orthonormal, see \eqref{eq:p-orthogonality}. The
polynomials are defined as $\jpoly{-1}{\alpha}{\beta}\equiv 0$ and
$\jpoly{0}{\alpha}{\beta} = \frac{1}{\sqrt{b_0^{(\alpha,\beta)}}}$. The
following are well-known Jacobi polynomial identities for $n,m\in \N$,
$\alpha,\beta>-1$, and $\theta = \arccos r$:
\begin{subequations}
\begin{align}
  \label{eq:p-3term-recurrence} \sqrt{b^{(\alpha,\beta)}_n}
    \jpoly{n}{\alpha}{\beta}(r) &= 
    (r - a^{(\alpha,\beta)}_{n-1}) \jpoly{n-1}{\alpha}{\beta}(r) - 
    \sqrt{b^{(\alpha,\beta)}_{n-1}} \jpoly{n-2}{\alpha}{\beta}(r) \\
  \label{eq:p-orthogonality}
    \langle \jpoly{n}{\alpha}{\beta}, \jpoly{m}{\alpha}{\beta}
    \rangle_{(\alpha,\beta)} &= \delta_{m,n} \\
  \label{eq:p-symmetry}
    \jpoly{2n}{\alpha}{\alpha} (-r) &= \jpoly{2n}{\alpha}{\alpha} (r)  \\
  \label{eq:p-ultraspherical}
    \jpoly{2 n}{1/2}{1/2}\left(\sqrt{\frac{r+1}{2}}\right) &= \sqrt{2}
    \jpoly{n}{1/2}{-1/2}(r) \\
  \label{eq:p-connection1}
    \jpoly{n}{\alpha}{\beta} &= \nu_{n,0}^{(\alpha,\beta)} \jpoly{n}{\alpha}{\beta+1} +
      \nu_{n,-1}^{(\alpha,\beta)} \jpoly{n-1}{\alpha}{\beta+1} \\
  \label{eq:u-sin-relation}
    U_n(r) &\doteq \sqrt{\frac{\pi}{2}} 
    \jpoly{n}{1/2}{1/2}(r) = \frac{\sin ((n+1) \theta)}{\sin \theta} \\
  \label{eq:t-product}
    \jpoly{m}{-1/2}{-1/2} \jpoly{n}{-1/2}{-1/2} &= \frac{1}{\sqrt{2\pi}}
    \left(\jpoly{m+n}{-1/2}{-1/2} + \jpoly{|m-n|}{-1/2}{-1/2}\right) \\
  \label{eq:u-product} U_n U_m &= \sum_{j=0}^{m} U_{n-m+2j}  \hskip 20pt \textrm{(assuming $n\geq m$)}
\end{align}
\end{subequations}
All the constants $a_n^{(\alpha,\beta)}$, $b_n^{(\alpha,\beta)}$,
$\nu_{n,0}^{(\alpha,\beta)}$, and $\nu_{n,-1}^{(\alpha,\beta)}$ are known, 
computable, and have closed-form expressions. In \eqref{eq:t-product}, any term
with a $p_0$ must be multiplied by $\sqrt{2}$.
\begin{lemma} For any $k>0$,
  \begin{align*}
    U_{k-1}^4\left(\sqrt\frac{r+1}{2}\right) \doteq h_{k-1} = \sum_{j=0}^{2k-2} \hat{h}^{(-1/2,
    -1/2)}_j \jpoly{j}{-1/2}{-1/2},
  \end{align*}
  where
  \begin{align*}
   \hat{h}^{(-1/2,-1/2)}_j = \left\{\begin{array}{ll}
     \frac{\sqrt{\pi}}{3} k (2k^2+1), & j=0, \\[8pt]
     \sqrt{\frac{\pi}{2}}(j^3 - 2 j^2 k - j + \frac{4}{3} k^3 + \frac{2}{3} k), & 1\leq j\leq k, \\[8pt]
     \frac{1}{3}\sqrt{\frac{\pi}{2}} (2k-j-1)(2k-j)(2k-j+1), & k+1\leq j \leq 2 k -2.
   \end{array}\right.
  \end{align*}
\end{lemma}
\begin{proof}
Usage of \eqref{eq:u-product} and \eqref{eq:p-ultraspherical} gives
  \begin{align*}
    U^4_{k-1}\left(\sqrt\frac{1+r}{2}\right) = \pi (f_{k-1})^2,
  \end{align*}
where $f_{k-1} = \sum_{j=0}^{k-1} \jpoly{j}{1/2}{-1/2}$. Invert a linear system
defined by \eqref{eq:p-connection1} to obtain
\begin{align*}
 f_{k-1} = \sum_{j=0}^{k-1} \jpoly{j}{1/2}{-1/2} = \sum_{j=0}^{k-1}
 \jpoly{j}{-1/2}{-1/2},
\end{align*}
where 
\begin{align*}
  \hat{f}^{(-1/2,-1/2)} = \left\{\begin{array}{ll}
     k, & j=0, \\
     \sqrt{2}(k-j), & 1 \leq j \leq k-1,
  \end{array}\right.
\end{align*}
Now use \eqref{eq:t-product} on the $(\alpha,\beta) = (1/2,1/2)$ expansion of
$f^2_{k-1}$ to obtain the result.
\end{proof}
\begin{lemma} Define the integral 
\begin{align*}
  J_p^\alpha(k) = 2\int_{-1}^1 U_{k-1}^4(r) |r|^{2 \alpha +1} (1-r^2)^{1-\alpha}
  \dx{r}.
\end{align*}
Then 
\begin{align*}
   J_p^{1/2} &= \pi\left(k - \frac{3}{4}\right), \\
   J_p^{3/2} &= \pi\left(\frac{4}{3}k^3 - \frac{4}{3} k + \frac{3}{4}\right).
\end{align*}
\end{lemma}
\begin{proof}
  It is clear that $J_p^\alpha(0) \equiv 0$.
  Therefore we only consider $k > 0$. Using first the symmetry relation
  \eqref{eq:p-symmetry} and then the substitution $r \gets
  \sqrt{\frac{r+1}{2}}$, we obtain
  \begin{align*}
    J_p^\alpha(k) = \frac{1}{2} \int_{-1}^1
    U^4_{k-1}\left(\sqrt{\frac{r+1}{2}}\right) \omega^{(1-\alpha,\alpha)}
    \dx{r}.
  \end{align*}
  Usage of \eqref{eq:u-product} and \eqref{eq:p-ultraspherical} then gives
  \begin{align*}
    J_p^\alpha(k) = \frac{\pi}{2} \langle f_{k-1}, f_{k-1}
    \rangle_{(1-\alpha, \alpha)},
  \end{align*}
  where $f_{k-1} = \sum_{j=0}^{k-1} \jpoly{j}{1/2}{-1/2}$. In order to arrive at
  the result for $\alpha = \frac{1}{2}$ we use \eqref{eq:p-connection1} to
  establish that
  \begin{align*}
    f_{k-1} = \sum_{j=0}^{k-1} \jpoly{j}{1/2}{-1/2} = \sqrt{2} \sum_{j=0}^{k-2}
      \jpoly{j}{1/2}{1/2} + \frac{1}{\sqrt{2}} \jpoly{k-1}{1/2}{1/2}.
  \end{align*}
  With $f_{k-1}$ expanded in a $(\alpha,\beta) = (1/2,1/2)$ orthogonal series, it is easy to
  use \eqref{eq:p-orthogonality} to compute that
  \begin{align*}
    J_p^{1/2}(k) = \frac{\pi}{2} \| f_{k-1} \|^2_{(1/2,1/2)} = \frac{\pi}{2}
    \left( 2(k-2) + \frac{1}{2}\right) = \pi\left(k - \frac{3}{4}\right).
  \end{align*}
  Now consider $\alpha = \frac{3}{2}$; inverting a linear system defined by
  \eqref{eq:p-connection1}, and then employing \eqref{eq:p-3term-recurrence} we
  can deduce
  \begin{align*}
     (1+r) f_{k-1} &= (1+r) \sum_{j=0}^{k-1} \jpoly{j}{1/2}{-1/2} \\
     & = (1+r) \sum_{j=0}^{k-1}
      \hat{f}^{(-1/2,-1/2)} \jpoly{j}{-1/2}{-1/2} \\
     &= \sum_{j=0}^k \hat{g}^{(-1/2,-1/2)} p_j^{(-1/2,-1/2)},
  \end{align*}   
  where 
  \begin{align*}
  \hat{f}^{(-1/2,-1/2)} = \left\{\begin{array}{ll}
     k, & j=0, \\
     \sqrt{2}(k-j), & 1 \leq j \leq k-1,
  \end{array}\right. & &
  \hat{g}^{(-1/2,-1/2)} = \left\{\begin{array}{ll}
     (2k-1), & j=0, \\
     2\sqrt{2}(k-j), & 1 \leq j \leq k-1, \\
     \frac{1}{\sqrt{2}}, & j=k.
  \end{array}\right.
  \end{align*}
  Now we observe that 
  \begin{align*}
    \frac{2}{\pi} J^{3/2}_p(k) = \left\langle f_{k-1}, f_{k-1} \right\rangle_{(-1/2,
    3/2)} = \left\langle (1+r) f_{k-1}, (1+r) f_{k-1} \right\rangle_{(-1/2,
    -1/2)},
  \end{align*}
  and since we have the $(-1/2, -1/2)$ expansion coefficients of $(1+r) f_{k-1}
  = g$, then \eqref{eq:p-orthogonality} yields
  \begin{align*}
    J^{(3/2)}_p(k) = \frac{\pi}{2} \left\| (1+r) f_{k-1} \right\|_{(-1/2,-1/2)} =
    \pi\left(\frac{4}{3} k^3 - \frac{4}{3} k + \frac{3}{4}\right).
  \end{align*}
\end{proof}
The above lemma basically states that $J_p^\alpha(k) \sim k^{2 \alpha}$ for
certain values of $\alpha$. Because
the proof relies almost entirely on `trigonometric' Jacobi polynomials (those
with $\alpha,\beta = \frac{2n-1}{2}$ for $n \in \N_0$), the
proof would also follow from use of various trigonometric identities; however,
the above method seems easier.
\begin{comment}
      \begin{lemma} The Chebyshev polynomials of the second kind also satisfy
       \begin{align*}
         8 \int_{-1}^1 r^2 U_n^4 \omega_U \dx{r} = (2n + 1) \pi
       \end{align*}
      \end{lemma}
      \begin{proof}
        Both identities are easily proven using relations
        \eqref{eq:u-3term-recurrence} - \eqref{eq:u-orthogonality}:
        \begin{align*}
          8 \int_{-1}^1 r^2 U_k^4 \omega_U \dx{r} &= 8 \int_{-1}^1 r^2 \left(
          \sum_{m=0}^n U_{2 m} \right)^2 \omega_U \dx{r} \\
          &= 2 \left\langle \sum_{m=0}^n \left(U_{2m-1} + U_{2m+1}\right), 
                     \sum_{m=0}^n \left(U_{2m-1} +
                     U_{2m+1}\right)\right\rangle_{\omega_U} \\
          &= (2n+1) \pi
        \end{align*}
      \end{proof}
\end{comment}
A non-periodic Stein integral was defined as
\begin{align}\label{eq:stein-integral}
  S^\alpha[v] = \int_{-\infty}^{\infty} \int_0^{2\pi} |v(\theta + s) + v(\theta - s)
  - 2 v(\theta)|^2 \frac{1}{s^{2\alpha+1}} \dx{s}\dx{\theta}.
\end{align}
Now define a periodic version of a Stein integral:
\begin{align}\label{eq:stein-integral-periodic}
  S^\alpha_p [v] = \int_0^{2\pi} \int_0^{2\pi} |v(\theta + s) + v(\theta - s)
  - 2 v(\theta)|^2 \left| \cot \left(\frac{s}{2}\right)\right|^{2\alpha+1} \dx{s}\dx{\theta}.
\end{align}
The lemmas proven above allow a quick proof of our desired result.
\begin{theorem}\label{thm:wp-periodic-stein}
  For a smooth $v$, the $W P$ norm is given by 
  \begin{align*} 
    \|v \|^2_{W P} &= \frac{3}{128\pi}\left( S^{3/2}_p[v] - S^{-1/2}_p [v] \right) \\
                 &= \frac{3}{128\pi} \int_0^{2\pi} \int_0^{2\pi} |v(\theta + s) + v(\theta - s)
  - 2 v(\theta)|^2 \left(\cot^4 \left(\frac{s}{2}\right) - 1\right)\dx{s}\dx{\theta}.
  \end{align*}
\end{theorem}
\begin{proof}
  When $\alpha = -\frac{1}{2}$ then Plancherel's Theorem immediately gives
  \begin{align*}
  S^{-1/2}_p[v] &= \int_0^{2\pi} \int_0^{2\pi} |v(\theta+s) + v(\theta-s) - 2
  v(\theta)|^2 \dx{s}\,\dx{\theta} \\
  &= 4\sum_{k\in \Z} |\hat{v}_k|^2 \int_0^{2\pi} |cos (sk) - 1|^2 \dx{s} \\
  &= 12 \pi \|v\|^2
  \end{align*}
  A similar calculation for general $\alpha$ yields
  \begin{align*}
    S_p^{\alpha}[v] &= \int_0^{2\pi} \int_0^{2\pi} |v(\theta+s) + v(\theta-s) - 2
    v(\theta) |^2 \left|\cot \left(\frac{s}{2}\right)\right|^{2\alpha+1} \dx{s} \dx{\theta} \\
    &= 16 \sum_{k \in \Z} \left| \hat{v}_k \right|^2 \int_0^{2\pi}
      \frac{\sin^4\left(\frac{s k}{2}\right)}{\sin^4\left(\frac{s}{2}\right)}
      \left| \cos\frac{s}{2}\right|^{2\alpha+1} \left|
      \sin\frac{s}{2}\right|^{3-2\alpha} \dx{s} \\
    &= 16 \sum_{k \in \Z} \left| \hat{v}_k\right|^2 2 \int_{-1}^1 U_{|k|-1}^4(r)
    |r|^{2 \alpha+1} (1-r^2)^{1-\alpha} \dx{r},
  \end{align*}
  where the last equality uses \eqref{eq:u-sin-relation} with the substitution $r
  \gets \cos \frac{s}{2}$. Now we have determined that
  \begin{align*}
    S_p^{3/2}[v] &= 16\sum_{k \in \Z} \left| \hat{v}_k\right|^2 J_p^{3/2} (|k|) \\
               &= \frac{64\pi}{3} \left\| v^{(3/2)} \right\|^2 - \frac{64\pi}{3}
               \left\| v^{(1/2)} \right\|^2 + 12 \pi \|v \|^2
  \end{align*}
  Usage of this and \eqref{eq:wp-norm-fourier} gives the result.
  \begin{comment}
        \begin{align*}
          S^{3/2}[v] &= \int_0^{2\pi} \int_0^{2\pi} |f(\theta+s) + f(\theta-s) - 2
          f(\theta) |^2 \cot^2\left(\frac{s}{2}\right) \dx{s} \dx{\theta} \\
          &= 4 \sum_{k \in \Z} \left| \hat{f}(k) \right|^2 \int_0^{2\pi} \left| 1 - \cos (k
          s) \right|^2 \cot^2\left(\frac{s}{2}\right) \dx{s} \\
          &= 16 \sum_{k \in \Z} |\hat{f}(k)|^2  \int_0^{2\pi} \frac{\sin^2\left(\frac{k
          s}{2}\right)} 
          {\sin^2\left(\frac{s}{2}\right)} \sin^2\left(\frac{k s}{2}\right)
          \cos^2\left(\frac{s}{2}\right) \dx{s} \\
          &= 32 \sum_{k \in \Z} |\hat{f}(k)|^2  \int_{-1}^1 r^2 U^4_{|k|-1}(r) \omega_U
          \dx{r} \\
          &= 4\pi \sum_{k \in \Z} |\hat{f}(k)|^2 (2(|k|-1) + 1) \\
          &= 8\pi \left\| f^{(1/2)} \right\|^2 - 4 \pi \| f \|^2
        \end{align*}
  \end{comment}
\end{proof}
