# Supplementary material for: Numerical Computation of Weil-Peterson Geodesics in the Universal Teichm\"uller Space
Source: arXiv:1307.2358 source file (2015-10-14)
Supplement: Supplementary file 2 [file appendix-stein-accuracy.tex]

\section{Computing Stein integrals}

Theorem \ref{theorem-fractional-derivatives} enables the computation of
Sobolev seminorms via direct point-evaluation quadrature. To facilitate the
computation of these quantities, we explicitly compute the constants $b_\alpha$
that connect the Stein double integral with the Sobolev seminorm. We recall
\eqref{eq:stein-formula}, and the proof of Theorem
\ref{theorem-fractional-derivatives} yields the following expression for these
constants:
\begin{align*}
  b_\alpha = 32 \int_0^\infty \frac{\sin^4\left(\frac{s}{2}\right)}{s^{1 + 2
  \alpha}} \dx{s}
\end{align*}
\sout{Now use Wolfram Alpha}. Clearly this expression is equal to 
\begin{align*}
  b_\alpha = \left\{ \begin{array}{lcl}
          4 \pi, & & \alpha = \frac{1}{2} \\
          8 \log{2}, & & \alpha = 1 \\
          \frac{4\pi}{3}, & & \alpha = \frac{3}{2} \\
          4\left(4^\alpha - 4\right) \cos({\pi \alpha}) \Gamma(-2 \alpha), & &
          \alpha \in (0,2)\backslash\left\{\frac{1}{2}, 1, \frac{3}{2}\right\}
  \end{array}\right.
\end{align*}

Corollary \ref{corollary-wp-norm} characterizes the WP norm in terms of
doubly-infinite (``Stein") integrals. In particular, it indicates that we will
need to accurately evaluate the integrals from Theorem
\ref{theorem-fractional-derivatives}. The main challenges for these integrals is
their unbounded nature (in the $s$ variable). For $f\in H^\alpha$ let us
consider how to evaluate integrals of the form 
\begin{align}\label{eq:stein-integral}
  I(f) = \int_0^{2\pi} \int_0^\infty \frac{\left|f(\theta+s) + f(\theta-s) - 2f(\theta)\right|^2}
                                          {s^{2\alpha+1}} \dx{s}\,\dx{\theta}.
\end{align}                                        

\subsection{A finite-element approach}
The Stein integrals \ref{eq:stein-integral} are challenging to compute
numerically, and we pose the following design requirements for the numerical
method we use:
\begin{itemize}
  \item The method should be able to handle smooth functions in a convergent
  manner. 
  \item We require a nonuniform grid formulation; velocity fields of interest
  frequently have derivatives of high magnitude. Using an equidistant grid
  results in a prohibitive number of points in order to properly resolve
  velocity fields.
  \item The method should have a tunable accuracy in both the $s$ integral and
  the $\theta$ integral.
  \item The number of function evaluations required for accuracy should be minimized.
\end{itemize}
To address all of these issues, we propose the following method: let $I^k$, $k
=1, 2, \ldots, K$ be a collection of disjoint closed intervals on $[0, 2\pi]$
such that $\cup I^k = [0, 2\pi]$; we further assume that the intervals are
ordered in $k$. For each interval, let $\{\theta^k_n, w^k_n\}_{n=1}^N$ be the local
$N$-point Legendre Gauss-Lobatto grid. Then for any $f \in L^2$
\begin{align*}
  \int_0^{2\pi} f(\theta) \dx{\theta} \simeq \sum_{k=1}^K \sum_{n=1}^{N_\theta}
  w^k_n f(\theta^k_n).
\end{align*}
This is the simple manner in which we will handle the $\theta$ integral. The
$s$ integral, being unbounded, is more difficult: let $I^k_n$ for $n=1, 2,
\ldots, N_\theta-1$ be the closed interval $[\theta^k_n, \theta^k_{n+1}]$. Then
$I^k = \cup_n I^k_n$. Given $N_s \in \N$, let $\{\theta^k_{n,m}\}$ be the
$N_s$-point Legendre-Gauss grid on $I^k_n$. Define 
\begin{align*}
  w^k_{n,m} = 
\end{align*}

\subsection{A symmetric staggered grid approach}
Our strategy relies on a staggered-grid aproach: we use canonical Fourier
quadrature for the $\theta$ integral and Gauss-Legendre quadrature for the $s$
integral. For $N_\theta \in \N$, define
\begin{align*}
  \theta_j = \frac{(2j+1)\pi}{N_\theta}, \hskip 10pt I_j = (\theta_j,
  \theta_{j+1}), \hskip 10pt j = \{1, 2, \ldots, N_\theta\}.
\end{align*}
Then for $N_s \in \N$,  let $\left\{r_k, w_k\right\}_{k=1}^{N_s}$ denote the
$N_s$-point Gauss-Legendre quadrature rule over $[-1, 1]$. Finally, define a new grid
that staggers the $\theta_j$:
\begin{align*}
  s_{j, k} = \theta_j + \frac{\bar{I}_j}{2} + \frac{\bar{I}_j}{2} r_k,
  \hskip 10pt j \in \{1, 2, \ldots, N_\theta\},\;\;
              k \in \{1, 2, \ldots, N_s\}.
\end{align*}
By construction, $\left\{s_{j,k}\right\}_k$ is a local quadrature rule on $I_j$.
We approximate the integrals in \eqref{eq:stein-integral} as
\begin{align}
  \nonumber I_f &\simeq \frac{2\pi}{N_\theta} \sum_{j=1}^{N_\theta} \int_0^\infty 
        \frac{\left|f(\theta_j+s) + f(\theta_j-s) - 2f(\theta_j)\right|^2} 
             {s^{2\alpha+1}} \dx{s} \\\label{eq:stein-rule-symmetric}
      &\simeq \frac{2\pi}{N_\theta} \sum_{j=1}^{N_\theta} \sum_{m=0}^{\infty}
        \sum_{l,k} \frac{w_k \left|{f}(\theta_j + s_{l,k} + 2\pi m)
                         + {f}(\theta_j - s_{l,k} - 2\pi m) 
                         - 2f(\theta_j)\right|^2}
                        {\left(\left[\left(s_{l,k} - \theta_j\right)
                        \textrm{ mod } 2\pi \right] + 2\pi m\right)^{2\alpha+1}}
\end{align}
The sum over $m$ represents continuous rotations periodically (since $s$ is
unbounded). The above expression looks unwieldy, but computationally once
function evaluations for $f$ have been computed for $m=0$, they can be reused
for all $m$. In implementation, one can precompute new weights $\tilde{w}_{j,k}$
that hold all information about the summation over $m$ and one must only
perform the $l, k,$ and $j$ sums for each $f$. In practice, the upper limit on
$m$ is truncated to some large value, say $M$, so that any additional rotations
produce $\mathcal{O}(\varepsilon_{tol})$ contribution to the augmented weights
$\tilde{w}$. 

In this way, we only use $(N_s + 1)N_\theta = N_{\textrm{total}}$ function evaluations to
compute the integral $I(f)$. Because the function $f$ (a velocity field) is not
trivial to compute, we must try to minimize the number of evaluations needed. A
straightforward comparison to make is to use a global Fourier approximation to
calculate the integral:
\begin{align*}
  I(f) \propto \left| f \right|^2_{\alpha} = \sum_{n}
  \left|n^{\alpha} \hat{f}_n \right|^2,
\end{align*}
where $\hat{f}_n$ is the Fourier coefficient corresponding to $e^{i n \theta}$
and the limits for $n$ range over appropriate values in $\Z$.  In practice the
coefficients are computed using a quadrature rule (or the FFT) using the
available function evaluations. For $N_{\textrm{total}}=700$ function evaluations
and $\alpha = \frac{1}{2}, \frac{3}{2}$ we plot the computed Sobolev seminorms
using both the Stein and canonical Fourier methods in Figure
\ref{fig:fourier-accuracy-exp-symmetric}. The quantity $\varepsilon_{rel}$ is the
relative error.
\begin{figure}
  \begin{center}
    \beginpgfgraphicnamed{images/fourier-accuracy-exp-symmetric}
      \input{tikz/fourier-accuracy-exp-symmetric}
    \endpgfgraphicnamed
  \end{center}
  \caption{Comparison between Stein integral computations and canonical Fourier
  computations for Sobolev seminorms of order $\frac{1}{2}$, (left) and
  $\frac{3}{2}$ (right). The computed seminorms (top) and the relative errors
  (bottom) are shown. The test functions are given by $f_k = e^{i k \theta}$.
  The computations use $N_{\textrm{total}} = 700$.}
  \label{fig:fourier-accuracy-exp-symmetric} 
\end{figure}

The Fourier method is exact below the Nyquist limit; however, once this limit is
exceeded, the resulting error is $\mathcal{O}(1)$. In contrast, the Stein method
is not exact for any mode $k$, but is very accurate for lower modes, and even
gives quite good agreement to the exact solution well past the Nyquist limit.
Unfortunately, the results shown in Figure
\ref{fig:fourier-accuracy-exp-symmetric} are not a faithful representation of
how well this method works. Consider performing the same experiment, but with
test functions $f_k = \cos k\theta$. The results are now shown in Figure
\ref{fig:fourier-accuracy-cos-symmetric}. The Stein method produces considerably
less attractive results for the same number of function evaluations. This can be
rationalized as follows: the method \ref{eq:stein-rule-symmetric} relies on an
equidistant $\theta$ grid. Because of this, the integration in the $\theta$
variable is still restricted by the Nyquist limit. In particular, certain modes
get aliased down to the zero function; this is shown by the periodic
oscillations in the Stein curve down to zero. This does not manifest in Figure
\ref{fig:fourier-accuracy-exp-symmetric} because the test function $f_k = e^{i
k\theta}$ will never be aliased down to $0$ (it will be aliased to a
constant, but it turns out that this doesn't matter). 

\aknote{Regarding the last comment, you can work out the Stein integral exactly
for e.g. cosine modes and you see that the $\theta$ integral must only be able
to integrate a constant accurately. Of course, if the function is aliased to the
zero function, this won't happen. However, if you have a {\it complex}
exponential, it is never aliased to zero; thus the $\theta$ integral correctly
captures information.

Note that this means that Stein integrals {\it are} in fact more well-suited to
what we want to do: i.e. the $\theta$ integral can be very coarse, all it has to
do is capture information about constants. The $s$ integral takes care of
information about the oscillatory nature of the function. Unfortunately, due to
this aliasing technicality about aliasing down to zero instead of the constant
function, you see the crappy results in Figure
\ref{fig:fourier-accuracy-cos-symmetric}. I'm not certain certain I can get around this.}

\begin{figure}
  \begin{center}
    \beginpgfgraphicnamed{images/fourier-accuracy-cos-symmetric}
      \input{tikz/fourier-accuracy-cos-symmetric}
    \endpgfgraphicnamed
  \end{center}
  \caption{Comparison between Stein integral computations and canonical Fourier
  computations for Sobolev seminorms of order $\frac{1}{2}$, (left) and
  $\frac{3}{2}$ (right). The computed seminorms (top) and the relative errors
  (bottom) are shown. The test functions are given by $f_k = \cos k \theta$.
  The computations use $N_{\textrm{total}} = 700$.}
  \label{fig:fourier-accuracy-cos-symmetric} 
\end{figure}

Some velocity fields `look' as if they're not $H^{3/2}$. Although we will
attempt to deal with such problems via multiple charts, we should obtain an
understanding of how the numerical method will act when presented with a
function whose smooth nature cannot be captured by the grid resolution. 

\begin{figure}
  \begin{center}
    \beginpgfgraphicnamed{images/hat-and-fprint-plot}
      \input{tikz/hat-and-fprint-plot}
    \endpgfgraphicnamed
  \end{center}
  \caption{Two test functions used: the periodic hat function (left) and a
  velocity field obtained as the initial guess from a shape evolution (right).
  The velocity field is a smooth periodic function; the gradient near the
  endpoints is very large.}
  \label{fig:hat-and-fprint-plot} 
\end{figure}

We consider a hat function shown in Figure \ref{fig:hat-and-fprint-plot}. Since
the $3/2$-derivative of a hat function is not in $L^2$, we do not expect
convergence of the computed $\alpha = \frac{3}{2}$ seminorm. Figure
\ref{fig:hat-accuracy-symmetric} shows the results of this test. Both the
Fourier and Stein methods agree fairly well for the $\alpha=\frac{1}{2}$ case;
the `exact' integral is computing with the Fourier method and
$N_{\textrm{total}} = 20,000$. However, there is no agreement between the two in
the $\alpha=\frac{3}{2}$ case; in particular, the Stein computation does not
even appear to stabilize. The Fourier method does not converge either, but again
convergence is not expected in this case.
 
\begin{figure}
  \begin{center}
    \beginpgfgraphicnamed{images/hat-accuracy-symmetric}
      \input{tikz/hat-accuracy-symmetric}
    \endpgfgraphicnamed
  \end{center}
  \caption{Comparison between Stein integral computations and canonical Fourier
  computations for Sobolev seminorms of order $\frac{1}{2}$, (left) and
  $\frac{3}{2}$ (right). The test function is the hat function from the left
  plot of Figure \ref{fig:hat-and-fprint-plot}.}
  \label{fig:hat-accuracy-symmetric} 
\end{figure}

We now consider another test function: we compute a fingerprint minus the
identity for a shape as shown in the right plot of Figure
\ref{fig:hat-and-fprint-plot}. This function has extremely high frequency
content. The computed Sobolev seminorms are shown in Figure
\ref{fig:fprint-accuracy-symmetric}. We see in this case that neither the
$\alpha = \frac{1}{2}$ nor the $\alpha=\frac{3}{2}$ seminorms agree in this
case. It is difficult to say which is more accurate here since the velocity
field is extremely difficult to resolve.

\aknote{Yeah, I realize this velocity field is a crappy test case...I need to
change it. However, I was curious and wanted to push limits.}

\begin{figure}
  \begin{center}
    \beginpgfgraphicnamed{images/fprint-accuracy-symmetric}
      \input{tikz/fprint-accuracy-symmetric}
    \endpgfgraphicnamed
  \end{center}
  \caption{Comparison between Stein integral computations and canonical Fourier
  computations for Sobolev seminorms of order $\frac{1}{2}$, (left) and
  $\frac{3}{2}$ (right). The test function is the velocity field from the right
  plot of Figure \ref{fig:hat-and-fprint-plot}.}
  \label{fig:fprint-accuracy-symmetric} 
\end{figure}

\subsection{A nonsymmetric tensor-product grid}
We now consider a more straightforward method to integrate
\ref{eq:stein-integral}: we suppose that the $\theta$ grid $\theta_j$ can be
nonuniform. Then on each $I_j$ we lay down a Gauss-Legendre finite-element grid.
I.e., we have 
\begin{align*}
  \int_0^{2\pi} f(\theta) \dx{\theta} \simeq \sum_{j=1}^{N_\theta}
  \sum_{k=1}^{N_p} w_{j,k} f(\theta_{j,k}),
\end{align*}
where $\{\theta_{j,k}\}_{k=1}^{N_p}$ is a local Gauss-Legendre quadrature rule.
Then for each $\theta_{j,k}$ we must compute an integral in $s$:
\begin{align*}
  \int_0^\infty f(\theta_{j,k}, s) \dx{s},
\end{align*}
and we do this by employing an $N_s$-point mapped Gauss-Legendre grid. If
$\{r_l, w_l\}$ is a standard $N_s$-point Gauss Legendre grid on $[-1,1]$, we
employ the map
\begin{align}\label{eq:finite-to-infinite-map}
  s = \frac{1+r}{1-r}
\end{align}
to obtain nodes $s_l$ and we augment the weights $w_l$ to contain information
about the Jacobian of map \eqref{eq:finite-to-infinite-map}. This completes the
algorithm, but the drawback here is that we cannot reuse function evaluations:
this methods requires a full $N_s \times N_\theta \times N_p$ function
evaluations. Since $N_s$ must be large ($\approx 50$) this will require a large
number of function evaluations for an accurate computation. 

Finally in order to choose a good nonuniform grid, we sample the function on an
equispaced grid, use an ENO procedure to approximate the derivative, and we use
the function $\rho = |\log | f' ||$ as a density function for samples. $\theta$
samples are then drawn using an inverse-CDF method.

\begin{figure}
  \begin{center}
    \beginpgfgraphicnamed{images/fourier-accuracy-cos-gauss}
      \input{tikz/fourier-accuracy-cos-gauss}
    \endpgfgraphicnamed
  \end{center}
  \caption{Comparison between Stein integral computations and canonical Fourier
  computations for Sobolev seminorms of order $\frac{1}{2}$, (left) and
  $\frac{3}{2}$ (right). The test functions are given by $f_k = \cos k \theta$.
  The Fourier computations use $N_{\textrm{total}} = N_\theta \times N_p = 400$.
  The Stein computations use $50\times 400 = 20000$ points.}
  \label{fig:fourier-accuracy-cos-gauss} 
\end{figure}

For cosine modes, we plot the accuracy of this method in Figure
\ref{fig:fourier-accuracy-cos-gauss}. Note that here we have a much more
accurate representation from the Stein integrals, but that is because they use
50 fold more points than the Fourier method. Therefore, the apparent
disadvantage of the Nyquist limit in Figure \ref{fig:fourier-accuracy-cos-gauss}
is not shown for an equal number of function evaluations.
