# Supplementary material for: Numerical Computation of Weil-Peterson Geodesics in the Universal Teichm\"uller Space
Source: arXiv:1307.2358 source file (2015-10-14)
Supplement: Supplementary file 3 [file appendix-wp-invariance.tex]

\section{Local invariance of the Weil-Peterson metric}
We recall that the WP norm is invariant under adjoint action:
\begin{align*}
  \|v \|_{WP} = \| Ad_\phi (v) \|_{WP}.
\end{align*}
Although this is a global statement, it \sout{is} {\bf seems to be} also true
locally. I.e. for any $\phi \in PSL_2(\R)$, define $w := Ad_w v$ and let $h$ be
the map on $[0, 2\pi]$ induced by $\phi$. Then:
\begin{align*}
\int_I L v \bar{v}\, \dx{\theta} = \int_{h^{-1}(I)} w, \bar{w}\, \dx{\theta}
\end{align*}
Consider the example furnished by the function
\begin{align*}
 v(\theta) = \cos k \theta
\end{align*}
We take $k=6$ and break up the global interval $[0, 2\pi]$ into subintervals:
\begin{align*}
  \begin{array}{cllll}
  [0,2\pi) = & [0,          & \pi/4)\hskip 5pt \cup & & (I_1) \\
             & [\pi/4,      & \pi/3)\hskip 5pt \cup & & (I_2) \\
             & [\pi/3,      & 6\pi/7)\hskip 5pt \cup & & (I_3) \\
             & [6\pi/7,     & 10\pi/9)\hskip 5pt \cup & & (I_4) \\
             & [10\pi/9,    & 4)\hskip 5pt \cup & & (I_5) \\
             & [4,          & 5)\hskip 5pt \cup & & (I_6) \\
             & [5,          & 5\pi/3)\hskip 5pt \cup & & (I_7) \\
             & [5\pi/3,     & 2\pi) & & (I_8)
  \end{array}
\end{align*}
On each subinterval we compute the `local' WP norm by integrating only over that
subinterval. For the adjoint map, we (randomly) pick element $h$, shown in Figure
\ref{fig:wp-adjoint-map-plot} along with its derivative. Under this map, the
function $L v$ and $L w$ are shown in Figure \ref{fig:wp-adjoint-lv-plot}. We
compute the following local WP norms:\vskip 10pt

\begin{figure}
  \begin{center}
    \beginpgfgraphicnamed{images/wp-adjoint-map-plot}
      \input{tikz/wp-adjoint-map-plot}
    \endpgfgraphicnamed
  \end{center}
  \caption{Plot of the particular choice of function $h$ induced from a member
  of $PSL_2(\R)$ (left). The derivative (right) is also plotted.}
  \label{fig:wp-adjoint-map-plot} 
\end{figure}

{\scriptsize
\begin{tabular}{r|l|l|l|l|l|l|l|l|}
  & $j=1$ & $j=2$ & $j=3$ & $j=4$ & $j=5$ & $j=6$ & $j=7$ & $j=8$ \\\hline
  $\int_{I_j} L v \,\bar{v} \,\dx{\theta}$ & 
       6.562500 & 2.187500 & 14.294392 & 5.519259 & 4.323949 & 8.678332 & 2.184068 & 8.750000 \\\hline
  $\int_{h^{-1}(I_j)} L w \,\bar{w} \,\dx{\theta}$ &
       6.562440 & 2.187501 & 14.294222 & 5.519101 & 4.323842 & 8.678229 &
       2.184058 & 8.750506\\\hline
\end{tabular}
}

\begin{figure}
  \begin{center}
    \beginpgfgraphicnamed{images/wp-adjoint-lv-plot}
      \input{tikz/wp-adjoint-lv-plot}
    \endpgfgraphicnamed
  \end{center}
  \caption{Plot of the function $L v$ (left) and $L w$ (right), where $w=Ad_\phi
  v$. The intevals $I_j$ (left) and $h^{-1}(I_j)$ (right) are delineated by vertical
  dotted lines.}
  \label{fig:wp-adjoint-lv-plot} 
\end{figure}

\vskip 5pt
\noindent One can see that indeed this invariance is manifest despite the great variation
in local behavior induced by $h$ as seen in Figure \ref{fig:wp-adjoint-lv-plot}.
